# Supplementary material for: On Parameterized Complexity of Binary Networked Public Goods Game
Source: arXiv:2012.01880 source file (2021-12-19)
Supplement: Supplementary file 1 [file Appendix1.tex]

\section{Bug and fix for Algorithm 2 of \cite{yu2020computing}} \label{appendix:treePSNE}
\begin{theorem}(Theorem 3 of \cite{yu2020computing})
When \GG(\VV,\EE) is a tree, it takes $O(d_{max}\cdot|\VV | + |\EE|)$
time to compute a $PSNE$ or conclude that one does not exist, where $d_max$ is the maximum degree of G.
\end{theorem}
\subsection{Algorithm 1,2, TreePSNE of \cite{yu2020computing}}
The aim is to determine the existence of a PSNE in a tree \GG. Let us define $n'_{Y =1}$ (resp. $n'_{Y =0}$ ) [equivalent terminolgy is $n'_Y$ conditioned on $x_Y$] as the number of node $Y$’s children that invest in a
PSNE of the associated subtree given that Y invests (resp. not invests). Algorithm 1 of \cite{yu2020computing} is used to compute conditional best-response table $T_Y$ for a leaf node $Y$ whose parent is $W$. Algorithm 2 of \cite{yu2020computing} is used to compute conditional best-response table $T_Y$ for an internal node $Y$ which has $k$ children whose conditional best-response tables are $U_1,\ldots,U_k$ and has a parent $W$. When $x_Y=x$(x is either 0 or 1), we denote the number of $Y's$ children that always choose to invest (resp. not invest) as $n^1_{Y=x}$(resp. $n^0_{Y=x}$). \cite{yu2020computing} computes the best response table of root $R$ of \GG in $O(n)$ using a slightly modified version of Algorithm 2 of \cite{yu2020computing}. Then using the conditional best-response tables of the nodes PSNE of \GG can be computed (refer to TreePSNE Algorithm of \cite{yu2020computing}) given that the tables are computed correctly (as shown in proof of Theorem 3 of \cite{yu2020computing}).
\begin{algorithm}[ht!]
	\caption{Algorithm 1 of \cite{yu2020computing}}
	\label{algo1}
	\begin{algorithmic}[1]
		\STATE \textbf{Input:}$\Delta g_Y(.),c_Y$
		\STATE \textbf{Initialize:}$T_Y$
		\FOR{($x_W,x_y)$ in (0,0),(0,1),(1,0),(1,1)}
		\IF{$x_Y=0$}
			\IF{$\Delta g_Y(x_W)\leq c_Y$}
			\STATE put $(x_W,x_Y)$ into $T_Y$
			\ENDIF
		\ELSIF{$x_Y=1$}
			\IF{$\Delta g_Y(x_W)\geq c_Y$}
			\STATE put $(x_W,x_Y)$ into $T_Y$
			\ENDIF
		\ENDIF
		\ENDFOR
		\IF{$T_Y=\phi$}
		\RETURN No PSNE exists
		\ELSE
		 \RETURN $T_Y$
		\ENDIF
		
	\end{algorithmic}
\end{algorithm}
\begin{algorithm}[ht!]
	\caption{Algorithm 2 of \cite{yu2020computing}}
	\label{algo2}
	\begin{algorithmic}[1]
		\STATE \textbf{Input:}$\Delta g_Y(.),c_Y,k$ and conditional best-response tables $T_{U_1},\ldots,T_{U_k}$
		\STATE \textbf{Initialize:}$T_Y$
		\STATE Compute $n^1_{Y=0},n^0_{Y=0},n^1_{Y=1},n^0_{Y=1}$
		\FOR{($x_W,x_y)$ in (0,0),(0,1),(1,0),(1,1)}
		\IF{$x_Y=0$}
			\FOR{$n'_{Y=0}$ in $\{n^1_{Y=0},\ldots,k-n^0_{Y=0}\}$}
			\IF{$\Delta g_Y(n'_{Y=0}+x_W)\leq c_Y$}
			\STATE put $(x_W,x_Y)$ into $T_Y$
			\ENDIF
			\ENDFOR
		\ELSIF{$x_Y=1$}
			\FOR{$n'_{Y=1}$ in $\{n^1_{Y=0},\ldots,k-n^0_{Y=0}\}$}
			\IF{$\Delta g_Y(n'_{Y=1}+x_W)\geq c_Y$}
			\STATE put $(x_W,x_Y)$ into $T_Y$
			\ENDIF
			\ENDFOR
		\ENDIF
		\ENDFOR
		\IF{$T_Y=\phi$}
		\RETURN No PSNE exists
		\ELSE
		\RETURN $T_Y$
		\ENDIF
	\end{algorithmic}
\end{algorithm}
\begin{algorithm}[ht!]
	\caption{TreePSNE Algorithm of \cite{yu2020computing}}
	\label{algoTreePSNE}
	\begin{algorithmic}[1]
		\STATE \textbf{Input:}a BNPG game $(\GG,\UU)$
		\STATE \textbf{Initialize:}$T_R$
		\STATE Compute a Depth-first order \OO(start with leaves and end with the root)
		\FOR{$Y$ in \OO}
		\IF{$Y$ is the root}
		\STATE Compute $n'_R$ conditioned on $x_R$
		\STATE Compute the best response of the root by a modified version of Algorithm 2
		\ELSIF{$Y$ is a leaf node}
		\STATE Compute the conditional best-response table $T_Y$ by Algorithm 1
		\STATE Pass $T_Y$ to its parent
		\ELSE
		\STATE Compute the conditional best-response table $T_Y$ by Algorithm 2
		\STATE Pass $T_Y$ to its parent 
		\ENDIF
		\ENDFOR
		\STATE Let $\widehat{\OO}$ be the reversed Depth-first order.
		\FOR{$Y$ in $\widehat{\OO}$}
		\IF{$Y$ is the root}
		\STATE Choose an action $x_R \in T_R$
		\STATE Determine the actions of its children by the best-responses tables passed from them.
		\ELSIF{$Y$ is a leaf node}
		\STATE Pass
		\ELSE
		\STATE Determine the actions of its children by the best-responses tables passed from them.
		\ENDIF
		\ENDFOR
		\RETURN: A PSNE consisting of  the actions of the nodes
	\end{algorithmic}
\end{algorithm}
\subsection{Bug}
In Algorithm 2 of \cite{yu2020computing}, in the steps 6 to 8, for every $n'_{Y=0}$ in the set $\{n^{1}_{Y=0},\ldots,k-n^{0}_{Y=0}\}$ they check whether $\Delta g_Y(n'_{Y=0}+x_W)\leq c_Y$ and if it is true then $(x_W,0)$ into $T_Y$. But we could be adding a pair $(x_W,0)$ even when one of the children say $u$ of $Y$ doesn't contain 0 as Y's respone in any of the pairs in the response table of $u$. This can lead into incorrect PSNE.
\subsection{Fix}\label{algo2:fix}
Avoid executing the steps 6 to 8 for a pair of type $(x_W,0)$ if exists a child $u_1$ of $Y$ such that it doesn't contain 0 as Y's respone in its response table of $u_1$. Similarly avoid executing the steps 12 to 14 for a pair of type $(x_W,1)$ if exists a child $u_2$ of $Y$ such that it doesn't contain 1 as Y's respone in any of the pairs in the response table. Make similar changes for the slightly modified version of Algorithm 2 of \cite{yu2020computing} which was used for root $R$.

\section{Bug and fix for Proposition 2 of \cite{yu2020computing}}
\subsection{Bug}
Proposition 2 of \cite{yu2020computing} was that there exists a PSNE in a complete graph if and only if $\exists 0< k\leq n$ such that $\alpha(k)\leq k\leq n-\beta(k)$ (where $\alpha(k):=|\{i|c_i<\Delta g_i(k-1)\}|$ and $\beta(k):=|\{i|c_i>\Delta g_i(k-1)\}|$). We provide a counter example to this proposition. Consider a complete graph \GG(\VV,\EE) with only 2 players $A$ and $B$.
Let us now define the best response policy for all the vertices in the graph \GG. Let $n_{v}$ denote the number of neighbours of vertex $v\in\mathcal{V}$ who choose $1$ as their response. Let $x_{v}$ denote the best response of a vertex $v\in\mathcal{V}$ for a given value of $n_{v}$.

$ x_{A}= \left\{ \begin{array}{rcl}
1 & \mbox{for} & n_{A}=0  \\ 
0 & \mbox{for} & n_{A}=1 
\end{array}\right.$

 $x_{B}= \left\{ \begin{array}{rcl}
0 & \mbox{for} & n_{B}=0  \\ 
1 & \mbox{for} & n_{B}=1 
\end{array}\right.$
Consider the following of pair of responses $(x_A,x_B)$ and see whether there is any PSNE or not:
\begin{itemize}
\item (0,0): $A$ deviates to 1 and hence not a PSNE
\item (1,0): $B$ deviates to 1 and hence not a PSNE
\item (1,1): $A$ deviates to 0 and hence not a PSNE
\item (0,1): $B$ deviates to 0 and hence not a PSNE
\end{itemize}
So clearly we don't have a PSNE. But $\alpha(1)=1$ (as $\Delta g_A(0)>c_A$), $\beta(1)=1$ (as $\Delta g_B(0)<c_B$) and $\alpha(1)\leq 1\leq n-\beta(1)=1$. So it means that Proposition 2 of \cite{yu2020computing} is incorrect
\subsection{Fix}\label{prop2:fix}
Let us have a complete graph $G(V,E)$. $\forall k>0$ Let $\mathcal{S}(k)=\{i|c_i\geq \Delta g_i(k),\forall i\in V\}$. Let $\mathcal{R}(k)=\{i|c_i\leq \Delta g_i(k-1),\forall i\in V\}$ and $T(k)=|\mathcal{R}(k)|$ Then we have the following proposition:
\begin{proposition}
In a complete graph $G(V,E)$ there exists a PSNE where all the responses are not 0 if and only if $\exists 0< k\leq n:T(k)\geq k$, $|\mathcal{S}(k)|\geq |V|-k$ and $|\mathcal{S}(k)\setminus \mathcal{R}(k)|=|V\setminus \mathcal{R}(k)|$
\end{proposition}
\begin{proof}
If there exists a PSNE with $k>0$ responses as 1, then we have a set $\mathcal{K}_1$ of atleast $k$ players  such that $c_v\leq \Delta g_v(k-1)$ where $v\in \mathcal{K}_1$. So $T(k)\geq k$. Since $|V|-k$ players have their responses as 0 in the PSNE, it means that we have a set $\mathcal{K}_2$ of atleast $|V|-k$ players such that $c_v\geq \Delta g_v(k)$ where $v\in \mathcal{K}_2$. So $|\mathcal{S}(k)|\geq |V|-k$. Also for any player $v$ which doesn't belong to $\mathcal{R}(k)$, it's response is 0 which implies that $v\in \mathcal{S}(k)$. Hence we also have $|\mathcal{S}(k)\setminus \mathcal{R}(k)|=|V\setminus \mathcal{R}(k)|$.
\\ \\
In the other direction, let us assume that $\exists 0< k\leq n:T(k)\geq k$, $|\mathcal{S}(k)|\geq |V|-k$ and $|\mathcal{S}(k)\setminus \mathcal{R}(k)|=|V\setminus \mathcal{R}(k)|$. Let the response of all the players in $V\setminus \mathcal{R}(k)$ be 0 (all such players belong to $\mathcal{S}(k)$ otherwise $|V\setminus \mathcal{R}(k)|$ would have been greater than $|\mathcal{S}(k)\setminus \mathcal{R}(k)|$) . Choose $|V|-k-|V\setminus \mathcal{R}(k)|$ players from $\mathcal{R}(k)\cap\mathcal{S}(k)$ and make their response as 0. Note that this is possible as $|\RR(k)\cap\SS(k)|=|\SS(k)|-|V\setminus\RR(k)|\geq|V|-k-|V\setminus \mathcal{R}(k)|$ .Make responses of rest of the players as 1. Clearly players whose responses are 1 won't deviate as they belong to $\mathcal{R}(k)$ and players whose response are 0 won't deviate as they belong to $\mathcal{S}(k)$.

This concludes the proof of this proposition.
\end{proof}

We now propose the following Algorithm to check whether there is PSNE or not. First if $T(0)=n$ we have a PSNE where all the responses are 0. Otherwise we search for a $k$ greater than 0 and less than or equal to $n$ such that $T(k)\geq k$, $|\mathcal{S}(k)|\geq |V|-k$ and $|\mathcal{S}(k)\setminus \mathcal{R}(k)|=|V\setminus \mathcal{R}(k)|$. If there is no such $k$ we can conclude that there is no PSNE
\section{Bug and Fix in Theorem 8 of \cite{yu2020computing}}
A $k$-core of a graph \GG is a maximal induced subgraph \HH of \GG,
where each node in \HH has degree at least $k$.
\begin{theorem}(Theorem 8 of \cite{yu2020computing})
In a fully-homogeneous BNPG game with strictly convex function $g$ such that $\Delta g(k-1)<c<\Delta g(k)$, let $x$ be an action profile and \HH be the subgraph of \GG induced from the nodes corresponding to the investing players in $x$. If $x$ is a non-trivial PSNE, then \HH is a $k$-core of \GG.
\end{theorem}
\subsection{Bug}
Consider an undirected graph \GG with \VV=$\{v_1,v_2,\ldots,v_{k+3}\}$ and \\ \EE=$\{(v_i,v_j):1\leq i<j\leq k+1\}\cup \{(v_{k+2},v_i):1\leq i\leq k-1\} \cup \{(v_{k+3},v_i):1\leq i\leq k-1\} \cup (v_{k+2},v_{k+3})$. Let $\Delta g(k-1)<c<\Delta g(k)$.\\
\\
Consider the following response $X$ of the players :\\ $X=\{x_{v_i}=1:i\in[k+1]\}\cup\{x_{v_{k+2}}=0,x_{v_{k+3}}=0\}$. Clearly $\forall i\in[k+1]$, $v_i$ won't deviate as $n_v=k$. Also $v_{k+2}$ and $v_{k+3}$ won't deviate as $n_{k+2}=n_{k+3}=k-1$. But induced subgraph on $\{v_i:i\in[k+1]\}$ is not a k-core as the graph \GG is itself the k-core as degree of every vertex is atleast $k$
\subsection{Fix}
Now we claim that there can be exponentially many non trivial PSNE in this setting.  Consider the graph \GG mentioned in the previous subsection and make $n$ copies of it namely $\GG_1,\ldots,\GG_n$. $\forall i \in[n],\forall j\in[k+3]$, $v_j$ in \GG becomes $v_j^i$ in $\GG_i$. Now connect every vertex in the set $\{v_1^1,v_1^2,\ldots,v_1^n\}$ with each other by adding edge between each pair. Let us denote the resulting graph created by joining all the copies $\GG_1,\ldots,\GG_n$ as \GG'.  $\forall i \in [n]$, let $X_i^1=\{x_{v_j^i}=1:j\in[k+1]\}\cup\{x_{v_{k+2}^i}=0,x_{v_{k+3}^i}=0\}$ and $X_i^2=\{x_{v_j^i}=1:j\in[k+3]\}$. If  $\forall i\in[n]$ if the set of responses of players in $\GG_i$ is either $X_i^1$ or $X_i^2$, then we have a PSNE. Number of such PSNE is $2^n$ and out of that only one of them is a trivial PSNE.
